# Supplementary material for: Provable Reinforcement Learning with a Short-Term Memory
Source: arXiv:2202.03983 source file (2022-02-08)
Supplement: Supplementary file 1 [file app_eluder.tex]

Let $\Pi$ be set of all $m$-step policies and let $\ell :\Pi \times \Fcal \mapsto \mathbb{R}$.

\begin{definition}[$\epsilon$-Independence] Let $\pi^1,\dots,\pi^n,\bar{\pi}$ be polices in $\Pi$. We say $\bar{\pi}$ is $\epsilon$-independent with respect to loss function $\ell$ and function class $\Fcal$, if there exists $f \in \Fcal$ such that $\sqrt{\sum_{i=1}^n [\ell(\pi^i,f)]^2} \leq \epsilon$, but $|\ell(\bar{\pi},f)| > \epsilon$.  
\end{definition}

\begin{definition}[Eluder Dimension] The \emph{Eluder Dimension} $\dim_{\ell}(\Fcal,\epsilon)$, is the length of the longest sequence of $m$-step polices $\{\pi^1,\dots,\pi^n\}$, such that there exists $\epsilon' \geq \epsilon$ where $\pi^i$ is $\epsilon'$-independent of $\{\pi^i,\dots,\pi^{i-1}\}$ with respect to loss function $\ell$ and function class $\Fcal$, for all $i \in [n]$.
	
\end{definition}

\begin{proposition}[Akin to Proposition 11 in \citealt{jin2021bellman}]  
Suppose for loss function $\ell:\Pi \times \Fcal \mapsto \mathbb{R}$, we have
$
	\ell(\pi,f) = \langle \zeta (\pi) , \xi(f) \rangle,
$
	where $\zeta(\pi) , \xi(f) \in \mathbb{R}^{d}$ satisfying $\norm{\zeta(\pi)} \cdot \norm{\xi(f)} \leq \gamma$. Then we have,
	\begin{equation*}
		\dim_{\ell}(\Fcal,\epsilon) \leq \Ocal\big(1+d\log[1+\gamma/\epsilon^2]\big).
	\end{equation*}
\end{proposition}

\begin{lemma}[Akin to Lemma 41 in \citealt{jin2021bellman}]
	Given a loss function $\ell:\Pi \times \Fcal \mapsto [-C,C]$; Suppose $\{\pi^i\}_{i=1}^K \subseteq \Pi$ and $\{f^i\}_{i=1}^K \subseteq \Fcal$ satisfy that for all $k \in K$, $\sum_{i=1}^{k-1} [\ell(\pi^i,f^k)]^2 \leq \alpha$. Then for all $k \in [K]$ and $\omega > 0$, we have
	\begin{equation*}
		\sum_{i=1}^k | \ell(\pi^i,f^k) | \leq \Ocal\Big(\sqrt{\dim_{\ell}(\Fcal,\omega)\alpha k}+\min\{k,\dim_{\ell}(\Fcal,\omega)\}\cdot C + k\omega).
	\end{equation*} 
\end{lemma}

\begin{proof}[Proof of \cref{thm:golf_regret}]
Denote 
\begin{equation}
	\dim^\star(\epsilon) \defeq \max_{h \in [H]} \dim_{\Ecal^\star_h}(\Fcal,\epsilon)
\end{equation}	

By \cref{lem:golf_property} and \cref{prop:bellman_to_eluder}, we have
\begin{equation*}
	\dim^\star(\epsilon) \leq \mathcal{O}(S\log[S/\epsilon]).
\end{equation*}
We know that $\sum_{i=1}^{k-1} [\Ecal_h^\star(\pi^i,f^k)]^2 \leq A^m \beta$, Therefore if we invoke \cref{lem:eluder_main} with 
\begin{equation*}
\begin{cases}
	\ell = \Ecal^\star_h, C=2,\\
	\alpha = A^m \beta, \omega = \frac{\epsilon}{H},\\
\end{cases}	
\end{equation*}
We obtain
\begin{equation*}
	\frac{1}{K}\sum_{h=1}^H\sum_{k=1}^K \Ecal^{\star}_h(\pi^k,f^k) \leq \Ocal\Big(\sqrt{A^m \beta \dim^\star(\epsilon/H)}+\frac{\epsilon}{H}\Big)
\end{equation*}
\end{proof}
