# Supplementary material for: Provable Reinforcement Learning with a Short-Term Memory
Source: arXiv:2202.03983 source file (2022-02-08)
Supplement: Supplementary file 2 [file app_olive.tex]

\section{Proof sketch}

\paragraph{Moment Matching Policy.}  
Let $z_h= \cbr{x_{h}}\cup \cbr{x_{h-1},a_{h-1},..,x_{h-n},a_{h-n}}$ be the sequence of last $n$ previous observations. We define the \emph{moment matching policy} as follows.
\begin{align}
\pi_{f,h}( a \mid \phi^\star(z_h)) = \Pr_{\pi_f,h}[ a \mid \phi^\star(z_n)]. 
\end{align}

\paragraph{Extended Bellman Error.} We define the following notion of extended Bellman error.
\begin{align*}
    \Ecal_h\rbr{\pi_1,\pi_2,f} = \EE_{z_h\sim \pi_1\circ_{h-n-1} \pi_2}\sbr{f(z_h,\pi_{f}(z_h)) - r_h - f(z_{h+1},\pi_{f}(z_{h+1}))}.
\end{align*}
In words, the sequence of last $n$ observations at time step $h$ is sampled by executing the policy $\pi_1$ for $h-n-1$ time steps, and then, executing $\pi_2$ for $n$ time steps.

\paragraph{$Q^\star$ is not eliminated.} Assume that $Q^\star\in \Bcal^{k-1}$. Then, conditioning on the good event, $Q^\star$ is not eliminated. First, observe that for any $\pi$ and $\pi_f$ it holds that $\Ecal_h\rbr{\pi_f,\pi,Q^*}=0.$
\begin{align*}
    &\Ecal_h\rbr{\pi_f,\pi,Q^*} = \EE_{z_h\sim \pi_f\circ_{h-n} \pi}\sbr{Q^\star(z_h,\pi_{Q^\star}(z_h)) - r_h - Q^\star(z_{h+1},\pi_{Q^\star}(z_{h+1}))}\\
    &=\EE_{z_h\sim \pi_f\circ_{h-n} \pi}\sbr{V^\star(s_h(z_h)) - r_h - \max_{a}Q^\star(s_h(z_h),\pi_{Q^\star}(s_h))}=0,
\end{align*}
since $Q^\star$ satisfies the Bellman equation. Conditioning on the good event it holds that 
\begin{align*}
    \abr{\Ecal_h\rbr{\pi_f,\pi,Q^*} - \widehat{\Ecal}_h\rbr{\pi_f,\pi,Q^*}}\leq \epsilon
\end{align*}
since $Q^\star\in \Bcal^{k-1}$, which implies that
\begin{align*}
    \abr{\widehat{\Ecal}_h\rbr{\pi_f,\pi,Q^*}} \leq \epsilon,
\end{align*}
and, thus,  assuming that $Q^\star\in \Bcal^{k-1}$ and conditioning on the good event for the $k^{th}$ iteration, it holds that $Q^\star$ is not eliminated.

\paragraph{Performance difference lemma.}
Assume that $Q^\star\in \Bcal^{k-1}.$ This implies that the algorithm is optimistic, and, specifically, that $f^k(x_1,\pi_f(x_1))\geq V^\star(x_1)$. Applying the value difference lemma results with the following relations.

\begin{align}
    &V^\star - V^{\pi_k} \leq f^k(x_1,\pi_f(x_1)) - V^{\pi_k} \nonumber \\
    &=\sum_{h=1}^H \EE_{z_h\sim \pi_{f^k},a_h\sim \pi_{f^k}\rbr{\cdot | z_h}}\sbr{f^k(z_h,a_h) - r_h - f^k(z_{h+1},a_h)} \nonumber\\
    & = \sum_{h=1}^H \EE_{z_{h-n}\sim \pi_{f^k}}\sbr{\EE_{z_h\sim \PP_{\pi_{f^k}}\rbr{\cdot \mid \phi^\star(z_{h-n})},a_h\sim \pi_{f^k}\rbr{\cdot | z_h}}\sbr{f^k(z_h,\pi_f(z_h)) - r_h - f^k(z_{h+1},\pi_f(z_{h+1})) \mid \phi^\star(z_{h-n})}}. \label{eq: pd lemma consequence}
\end{align}
We now show that for any observation $z_h$ it holds that
\begin{align}
    \PP_{\pi_{f^k}}\rbr{z_h \mid \phi^\star(z_{h-n})} =  \PP_{\pi_{f^k,\phi^\star}}\rbr{z_h \mid \phi^\star(z_{h-n})}, \label{eq: what we need to prove moment matching policy}
\end{align}
i.e., conditioning on the latent state at time step $h-n$ and then executing $\pi_f$ is equivalent to conditioning on the latent state at time step $h-n$ and executing the corresponding moment-matching policy $\pi_{f,\phi}$.

By the Block assumption we can identify $z_h$ with a unique latent state. Thus,
\begin{align}
    \PP_{\pi_{f^k}}\rbr{z_h \mid \phi^\star(z_{h-n})} = q(z_h \mid \phi^\star(z_{h}))\PP_{\pi_{f^k}}\rbr{\phi^\star(z_{h}) \mid \phi^\star(z_{h-n})}. \label{eq: what we need to prove moment matching policy relation 1}
\end{align}
For convenience we denote $s_t \equiv \phi^\star(z_{t}).$ We get that
\begin{align*}
    &\PP_{\pi_{f^k}}\rbr{s_h \mid s_{h-n}}\\
    &=\sum_{s_{h-1}} \PP_{\pi_{f^k}}\rbr{s_h \mid s_{h-1}, s_{h-n}} \PP_{\pi_{f^k}}\rbr{s_{h-1} \mid s_{h-n}}\tag{Bayes' rule \& law of total probability}\\
    &=  \sum_{s_{h-1}} \PP_{\pi_{f^k}}\rbr{s_h \mid s_{h-1}} \PP_{\pi_{f^k}}\rbr{s_{h-1} \mid s_{h-n}} \tag{Markovian assumption of model}\\
    & = \sum_{s_{h-1},a_{h-1}} T\rbr{s_h \mid s_{h-1},a_{h-1}}\PP_{\pi_f}(a_{h-1}\mid s_{h-1}) \PP_{\pi_{f^k}}\rbr{s_{h-1} \mid s_{h-n}} \tag{Bayes' rule \& law of total probability}\\
    &\vdots\\
    & = \sum_{s_{h-1},a_{h-1},\ldots, s_{h-n},a_{h-n}} \prod_{t=n-h}^h T\rbr{s_t \mid s_{t-1},a_{t-1}}\PP_{\pi_f}(a_{t-1}\mid s_{t-1})\\
    & = \sum_{s_{h-1},a_{h-1},\ldots, s_{h-n},a_{h-n}} \prod_{t=n-h}^h T\rbr{s_t \mid s_{t-1},a_{t-1}}\pi_{\pi_f,\phi^\star}(a_{t-1}\mid \phi^\star(z_{t-1}))\\
    & = \PP_{\pi_{f^k,\phi^\star}}\rbr{s_h \mid s_{h-n}},
\end{align*}
where the last relation holds by repeating the same argument backwards. Plugging this back to~\eqref{eq: what we need to prove moment matching policy relation 1} establishes~\eqref{eq: what we need to prove moment matching policy}.

Plugging this back to~\eqref{eq: pd lemma consequence} we get that
\begin{align*}
    &V^\star - V^{\pi_k} \leq \sum_{h=1}^H \EE_{z_{h-n}\sim \pi_{f^k}}\sbr{\EE_{z_h\sim \PP_{\pi_{f^k}}\rbr{\cdot \mid \phi^\star(z_{h-n})},a_h\sim \pi_{f^k}\rbr{\cdot | z_h}}\sbr{f^k(z_h,\pi_f(z_h)) - r_h - f^k(z_{h+1},\pi_f(z_{h+1})) \mid \phi^\star(z_{h-n})}}\\
    & = \sum_{h=1}^H \EE_{z_{h-n}\sim \pi_{f^k}}\sbr{\EE_{z_h\sim \PP_{\pi_{f^k,\phi^\star}}\rbr{\cdot \mid \phi^\star(z_{h-n})},a_h\sim \pi_{f^k}\rbr{\cdot | z_h}}\sbr{f^k(z_h,\pi_f(z_h)) - r_h - f^k(z_{h+1},\pi_f(z_{h+1})) \mid \phi^\star(z_{h-n})}}\\
    & = \sum_{h=1}^H \EE_{z_{h-n}\sim \pi_{f^k}\circ_{h-n} \pi_{f^k,\phi^\star}}\sbr{f^k(z_h,\pi_f(z_h)) - r_h - f^k(z_{h+1},\pi_f(z_{h+1}))}
\end{align*}

\paragraph{Eliptical potential argument.} Define the sufficient-statistics matrix
\begin{align*}
    \sbr{X_h}_{\pi,f} = \Ecal\rbr{\pi,f, \phi^\star, h}.
\end{align*}
How can we assure that we eliminate a direction in each iteration (in the exact case?).

Because we have the telescoping decomposition:
\begin{align*}
    V^\star - V^{\pi_k} \leq V^{f_k} - V^{\pi_k} = \sum_{h=1}^H \Ecal(\pi_k, f_k, \phi^\star, h)
\end{align*}
